# Supplementary material for: SV3D: Novel Multi-view Synthesis and 3D Generation from a Single Image using Latent Video Diffusion
Source: arXiv:2403.12008 source file (2024-03-18)
Supplement: Supplementary file 1 [file B.tex]

\section{Related Work}
\label{supsec:related_work}

\textbf{Video Synthesis.} 
%Due to its computational demands, 
%and a lack of publicly available data, 
%video synthesis has not been among the most investigated research areas for several years. However, 
Many approaches based on various models such as variational RNNs~\cite{babaeizadeh2018stochastic,svg,lee2018savp,hvrnn,lsvg}, normalizing flows~\citep{si2v,ipoke}, autoregressive transformers~\cite{Weissenborn2020Scaling,yan2021videogpt,hong2022cogvideo,wu2021godiva,wu2022nuwa,ge2022longvideo,Gupta_2022_CVPR}, and GANs~\citep{scene_dyn,yu2022generating,tian2021a, villegas17mcnet,Luc2020TransformationbasedAV,TGAN2020,brooks2022generating,Skorokhodov_2022_CVPR,kahembwe2020lower,TGAN2017,Wang_2020_CVPR,fox2021stylevideogan} have tackled video synthesis. Most of these works, however, have generated videos either on low-resolution~\citep{babaeizadeh2018stochastic,svg,lee2018savp,hvrnn,lsvg,si2v,ipoke,scene_dyn,yu2022generating,tian2021a, villegas17mcnet,Luc2020TransformationbasedAV} or on comparably small and noisy datasets~\cite{carreira2017quo,soomro2012ucf101,xu2016msr-vtt} which were originally proposed to train discriminative models. 

Driven by increasing amounts of available compute resources and datasets better suited for generative modeling such as WebVid-10M~\citep{bain2022frozen}, more competitive approaches have been proposed recently, mainly based on well-scalable, explicit likelihood-based approaches such as diffusion~\cite{ho2022video,singer2022make,ho2022imagenvideo} and autoregressive models~\citep{villegas2022phenaki}. Motivated by a lack of available clean video data, all these approaches are leveraging joint image-video training~\citep{singer2022make,ho2022imagenvideo,zhou2022magicvideo,blattmann2023align} and most methods are grounding their models on pretrained image models~\citep{singer2022make,zhou2022magicvideo,blattmann2023align}. Another commonality between these and most subsequent approaches to (text-to-)video synthesis~\cite{ge2023preserve,wang2023modelscope,wang2023lavie} is the usage of dedicated expert models to generate the actual visual content at a coarse frame rate and to temporally upscale this low-fps video to temporally smooth final outputs at 24-32 fps~\citep{singer2022make,ho2022imagenvideo,blattmann2023align}. Similar to the image domain, diffusion-based approaches can be mainly separated into cascaded approaches~\citep{ho2022imagenvideo} following~\citep{ho2021cascaded,ge2023preserve} and latent diffusion models~\citep{blattmann2023align,zhou2022magicvideo,zhang2023i2vgen} translating the approach of \citet{rombach2021high} to the video domain. While most of these works aim at learning general motion representation and are consequently trained on large and diverse datasets, another well-recognized branch of diffusion-based video synthesis tackles personalized video generation based on finetuning of pretrained text-to-image models on more narrow datasets tailored to a specific domain~\citep{guo2023animatediff} or application, partly including non-deep motion priors~\citep{zhang2023i2vgen}. Finally, many recent works tackle the task of image-to-video synthesis, where the start frame is already given, and the model has to generate the consecutive frames~\cite{zhang2023i2vgen,wang2023modelscope,guo2023animatediff}. Importantly, as shown in our work (see~\Cref{fig:teaser}) when combined with off-the-shelf text-to-image models, image-to-video models can be used to obtain a full text-(to-image)-to-video pipeline.

\textbf{Multi-View Generation}
Motivated by their success in 2D image generation, diffusion models have also been used for multi-view generation. Early promising diffusion-based results~\citep{watson2022novel,zhou2023sparsefusion,anciukevivcius2023renderdiffusion,nichol2022pointe,jun2023shape,deng2023nerdi} have mainly been restricted by lacking availability of useful real-world multi-view training data.     
To address this, more recent works such as Zero-123~\cite{liu2023zero1to3}, MVDream~\cite{shi2023mvdream}, and SyncDreamer~\cite{liu2023syncdreamer} propose techniques to adapt and finetune pretrained image generation models such as Stable Diffusion (SD) for multi-view generation, thereby leveraging image priors from SD.
% %% Multi-view generation problem and current techniques
% A typical 3D object reconstruction pipeline first involves capturing the multi-view images of an object followed by 3D optimization (e.g., NeRF~\cite{}).
% Following this protocol for generation, several recent works~\cite{zero123, zero123xl} propose techniques to 
% \textit{generate} multiple views of an object from a single image thereby facilitating the 3D asset generation from a given text or single object image. These works adapt the image generation models such as Stable Diffusion (SD)~\cite{} by adding a camera pose-conditioning thereby leveraging the generic image generation priors from SD. A typical strategy is to 
% fine-tune the image generation model on multi-view image datasets such as Objaverse~\cite{}. 
One issue with Zero-123~\cite{liu2023zero1to3} is that the generated multi-views can be inconsistent with respect to each other as they are generated independently with pose-conditioning. 
Some follow-up works try to address this view-consistency problem by jointly synthesizing the multi-view images. MVDream~\cite{shi2023mvdream} proposes to jointly generate four views of an object using a shared attention module across images. SyncDreamer~\cite{liu2023syncdreamer} proposes to estimate a 3D voxel structure in parallel to the multi-view image diffusion process to maintain consistency across the generated views.

%% Video models are more suitable for multi-view generation
Despite rapid progress in multi-view generation research, these approaches rely on single image generation models such as SD. We believe that our video generative model is a better candidate for the multi-view generation as multi-view images form a specific form of video where the camera is moving around an object. As a result, it is much easier to adapt a video-generative model for multi-view generation compared to adapting an image-generative model. In addition, the temporal attention layers in our video model naturally assist in the generation of consistent multi-views of an object without needing any explicit 3D structures like in~\cite{liu2023syncdreamer}.
