# Supplementary material for: SV3D: Novel Multi-view Synthesis and 3D Generation from a Single Image using Latent Video Diffusion
Source: arXiv:2403.12008 source file (2024-03-18)
Supplement: Supplementary file 2 [file C.tex]

\section{\textbf{Data Processing}}
\label{supsec:data_proc}
In this section, we provide more details about our processing pipeline including their outputs on a few public video examples for demonstration purposes. 
%All these visual examples are available on YouTube under a CC-license. We include the URL of each video example in the respective visualization.  

\paragraph{Motivation}
We start from a large collection of raw video data which is not useful for generative text-video (pre)training~\citep{ramesh2022hierarchical,wang2023internvid} because of the following adverse properties: First, in contrast to discriminative approaches to video modeling, generative video models are sensitive to motion inconsistencies such as cuts of which usually many are contained in raw and unprocessed video data, \cf \Cref{fig:cuts_and_motion}, left. Moreover, our initial data collection is biased towards still videos as indicated by the peak at zero motion in \Cref{fig:cuts_and_motion}, right. Since generative models trained on this data would obviously learn to generate videos containing cuts and still scenes, this emphasizes the need for cut detection and motion annotations to ensure temporal quality. Another critical ingredient for training generative text-video models are captions - ideally more than one per video~\citep{somepalli2023understanding} - which are well-aligned with the video content. The last essential component for generative video training which we are considering here is the high visual quality of the training examples.  

The design of our processing pipeline addresses the above points. Thus, to ensure temporal quality, we detect cuts with a cascaded approach directly after download, clip the videos accordingly, and estimate optical flow for each resulting video clip. After that, we apply three synthetic captioners to every clip and further extract frame-level CLIP similarities to all of these text prompts to be able to filter out outliers. Finally, visual quality at the frame level is assessed by using a CLIP-embeddings-based aesthetics score~\citep{schuhmann2022laion}. We describe each step in more detail in what follows.

% To instantiate our dataset we download the videos at native resolution, perform scene detection, and key-frame aware clipping \ref{keyframeaware}
% according to the detected scenes. The scene detection and clipping combination is useful for creating good quality video clips, however this creates the issue of losing unique metadata for each video since now we have multiple samples which come from the same base video and therefore share the same internet sourced metadata. One could use the subtitles that occur during a given clip as the text caption however this has its limitations. YouTube auto-generated subtitles are known to not have great quality and alignment and additionally audio transcripts rarely describe the \textit{visual} features that are occurring during a given time. To solve this issue we create synthetic captions which target visual and temporal descriptions for each clip. Additionally we collect the available YouTube metadata and compute and optical flow estimates for each clip. Below, we go into details on each of these transformations.
\cutsfadesvis

\paragraph{Cascaded Cut Detection.}
Similar to previous work~\citep{wang2023internvid}, we use PySceneDetect~\footnote{\url{https://github.com/Breakthrough/PySceneDetect}} to detect cuts in our base video clips. However, as qualitatively shown in \Cref{fig:cuts_fades} we observe many fade-ins and fade-outs between consecutive scenes, which are not detected when running the cut detector at a unique threshold and only native fps. Thus, in contrast to previous work, we apply a cascade of 3 cut detectors which are operating at different frame rates and different thresholds to detect both sudden changes and slow ones such as fades. 

% We clip the video frames with FFMPEG~\citep{tomar2006converting} directly after cut detection.

\paragraph{Keyframe-Aware Clipping.} We clip the videos using FFMPEG~\citep{tomar2006converting} directly after cut detection by extracting the timestamps of the keyframes in the source videos and snapping detected cuts onto the closest keyframe timestamp, which does not cross the detected cut. This allows us to quickly extract clips without cuts via seeking and isn't prohibitively slow at scale like inserting new keyframes in each video.

% We make use of the content-aware scene detection functionality of the PySceneDetect python package to detect scenes in videos and return their time ranges. This is parameterized by 2 arguments - a  threshold which controls the average change in pixel intensity required to trigger a cut and a minimum scene length (measured in frames). For our dataset, we chose to err on the side of caution, and set very aggressive thresholds for scene detection, choosing a threshold of 11.5. This has the effect of introducing unnecessary cuts in response to some motion, creating many extraneous small clips. So to combat this we filter all videos under 4 seconds long. % \todo{find info about those experiments we did early on and report here (I'm worried they might've had something to do with optical flow which was bad in those times)}

\staticvis
\paragraph{Optical Flow.} 
As motivated in \Cref{subsec:data_proc} and \Cref{fig:cuts_and_motion} it is crucial to provide means for filtering out static scenes. To enable this, we extract dense optical flow maps at 2 FPS using the OpenCV~\citep{itseez2015opencv} implementation of the Farneb\"ack algorithm~\citep{farneback2003flow}. To further keep storage size tractable, we spatially downscale the flow maps such that the shortest side is at 16px resolution. By averaging the flow vector magnitude over time and spatial coordinates, we further obtain a global motion score for each clip, which we use to filter out static scenes by using a threshold for the minimum required motion, which is chosen as detailed on \Cref{supsubsec:filtering_ablations}. Since this only yields rough approximate, for the final Stage III finetuning, we compute more accurate dense optical flow maps using RAFT~\cite{teed2020raft} at $800 \times 450$ resolution at 4 FPS. The motion scores are then computed similarly and scaled (divided) by a factor of 28.125 to match the distribution of pretraining data. Since the high-quality finetuning data is relatively much smaller than the pretraining dataset, this makes the RAFT-based flow computation tractable. Empirically, most motion score estimates computed by this method lie in the 0.0-3.5 range, with some scores over that. We divide this range of 0.0-3.5 into 1024 buckets and condition our model on the bucket ID where the motion scores lie, with values over 3.5 getting mapped to the last bucket.

% We use the OpenCV python package to compute the Gunnar-Farneback optical flow for each clip. In order to make this operation cheaper and metadata size smaller we downsample the input videos such that the shortest side is 16px, and we also temporally downsample to 2fps. We save the mean of the optical flow magnitudes across the spatial dimension and the entire video to produce a per-frame motion estimate and a per-clip motion estimate which can be easily used to filter the dataset based on desired amount of movement in videos. For example, one could set a minimal threshold for per-video optical flow mean and filter out videos with no motion in them. In fact we analyze this scenario in the next section.

\captionexamples
\paragraph{Synthetic Captioning.} At a million-sample scale, it is not feasible to hand-annotate data points with prompts. Hence we resort to synthetic captioning to extract captions. However in light of recent insights on the importance of caption diversity~\citep{somepalli2023understanding} and taking potential failure cases of these synthetic captioning models into consideration, we extract \emph{three} captions per clip by using i) the image-only captioning model CoCa~\citep{pucetti2023training}, which describes spatial aspects well, ii) - to also capture temporal aspects - the video-captioner VideoBLIP~\citep{videoblip} and iii) to combine these two captions and like that, overcome potential flaws in each of them, a lightweight LLM. Examples of the resulting captions are shown in \Cref{fig:captionextable}. Concurrent works~\citep{wang2023internvid} have also explored summarizing framewise image captions with an LLM, which could also be a reasonable alternative.

% We find that although the captioner was train on image captions which are often static it can produce relevant video captions which can be used to train capable video-text models. We briefly show this in the next section however we le ave a deeper analysis into synthetic captioning methods for future work.

\paragraph{Caption similarities and Aesthetics.} Extracting CLIP~\citep{radford2021learning} image and text representations have proven to be very helpful for data curation in the image domain since computing the cosine similarity between the two allows for assessment of text-image alignment for a given example~\citep{schuhmann2022laion} and thus to filter out examples with erroneous captions. Moreover, it is possible to extract scores for visual aesthetics~\citep{schuhmann2022laion}. Although CLIP is only able to process images, and this consequently is only possible on a single frame level we opt to extract both CLIP-based i) text-image similarities and ii) aesthetics scores of the first, center, and last frames of each video clip. As shown in \Cref{subsec:data_curation,supsubsec:filtering_ablations}, using training text-video models on data curated by using these scores improves i) text following abilities and ii) visual quality of the generated samples compared to models trained on unfiltered data.

\paragraph{Text Detection.} 
In early experiments, we noticed that models trained on earlier versions of \datasetfiltered obtained a tendency to generate videos with excessive amounts of written text depicted which is arguably not a desired feat for a text-to-video model. To this end, we applied the off-the-shelf text-detector CRAFT~\citep{baek2019character} to annotate the start, middle, and end frames of each clip in our dataset with bounding box information on all written text. Using this information, we filtered out all clips with a total area of detected bounding boxes larger than 7\% to construct the final \datasetfiltered. 
\ocrvis
% We found that at a large scale, lots of samples contained unwanted text like subtitles or unwanted graphic overlays. In an attempt to filter this, we used CRAFT text-detection~\citep{baek2019character} to annotate the beginning, middle, and end frame of each video with bounding box information on all text that might be present. From this we computed an area ratio which determines what percentage of each annotated frame is covered by text-boxes, and filtered out the worst-offending samples as in other experiments.  
