# Supplementary material for: SV3D: Novel Multi-view Synthesis and 3D Generation from a Single Image using Latent Video Diffusion
Source: arXiv:2403.12008 source file (2024-03-18)
Supplement: Supplementary file 3 [file D.tex]

\section{Model and Implementation Details} \label{supsec:model_and_implementation_details}
\subsection{Diffusion Models} \label{subsec:diffusion_models}
In this section, we give a concise summary of DMs. We make use of the continuous-time DM framework~\citep{song2020score,karras2022elucidating}. 
Let $\pdata(\rvx_0)$ denote the data distribution and let $p(\rvx; \sigma)$ be the distribution obtained by adding i.i.d. $\sigma^2$-variance Gaussian noise to the data. Note that or sufficiently large $\sigma_{\mathrm{max}}$, $p(\rvx; \sigma_{\mathrm{max}^2}) \approx \gN\left(\bm{0}, \sigma_{\mathrm{max}^2}\right)$. DM uses this fact and, starting from high variance Gaussian noise $\rvx_M \sim\gN\left(\bm{0},\sigma_{\mathrm{max}^2}\right)$, sequentially denoise towards $\sigma_0=0$. In practice, this iterative refinement process can be implemented through the numerical simulation of the \emph{Probability Flow} ordinary differential equation (ODE)~\citep{song2020score}
\begin{align} \label{eq:probability_flow_ode}
    d\rvx = -\dot \sigma(t) \sigma(t) \nabla_\rvx \log p(\rvx; \sigma(t)) \, dt,
\end{align}
where $\nabla_\rvx \log p(\rvx; \sigma)$ is the \emph{score function}~\citep{hyvarinen2005estimation}. DM training reduces to learning a model $\vs_\vtheta(\rvx; \sigma)$ for the score function $\nabla_\rvx \log p(\rvx; \sigma)$. 
The model can, for example, be parameterized as $\nabla_\rvx \log p(\rvx; \sigma) \approx s_\vtheta(\rvx; \sigma) = (D_\vtheta(\rvx; \sigma) - \rvx)/ \sigma^2$~\citep{karras2022elucidating}, where $D_\vtheta$ is a learnable \emph{denoiser} that tries to predict the clean $\rvx_0$. 
The denoiser $D_\vtheta$ is trained via \emph{denoising score matching}~(DSM)
\begin{align} \label{eq:diffusion_objective}
    \E_{\substack{(\rvx_0, \rvc) \sim \pdata(\rvx_0, \rvc), (\sigma, \rvn) \sim p(\sigma, \rvn)}} \left[\lambda_\sigma \|D_\vtheta(\rvx_0 + \rvn; \sigma, \rvc) - \rvx_0 \|_2^2 \right],
\end{align}
where $p(\sigma, \rvn) = p(\sigma)\,\gN\left(\rvn; \bm{0}, \sigma^2\right)$, 
$p(\sigma)$ can be a probability distribution or density over noise levels $\sigma$. 
It is both possible to use a discrete set or a continuous range of noise levels. In this work, we use both options, which we further specify in \Cref{subsec:base_model_training_and_architecture}.   

$\lambda_\sigma \colon \R_+ \to \R_+$ is a weighting function, and $\rvc$ is an arbitrary conditioning signal. In this work, we follow the EDM-preconditioning framework~\citep{karras2022elucidating}, parameterizing the learnable denoiser $D_\vtheta$ as
\begin{align} \label{eq:edm_preconditioning}
    D_\vtheta(\rvx; \sigma) = \cskip(\sigma) \rvx + \cout(\sigma) F_\vtheta(\cin(\sigma) \rvx; \cnoise(\sigma)),
\end{align}
where $F_\vtheta$ is the network to be trained.

\textbf{Classifier-free guidance.} Classifier-free guidance~\citep{ho2022classifier} is a method used to guide the iterative refinement process of a DM towards a conditioning signal $\rvc$. The main idea is to mix the predictions of a conditional and an unconditional model
\begin{align} \label{eq:guidance}
    D^w(\rvx; \sigma, \rvc) = w D(\rvx; \sigma,\rvc) - (w - 1) D(\rvx; \sigma),
\end{align}
where $w \geq 0$ is the \emph{guidance strength}. The unconditional model can be trained jointly alongside the conditional model in a single network by randomly replacing the conditional signal $\rvc$ with a null embedding in~\Cref{eq:diffusion_objective}, e.g., 10\% of the time~\citep{ho2022classifier}. In this work, we use classifier-free guidance, for example, to guide video generation toward text conditioning.

% \subsection{Architecture Details} %\label{supsec:arch} NO SUBSECTION REF ALLOWED FOR NOW

% \hyperparams
% Due to the recent success and computational efficiency of latent diffusion models (LDM)~\cite{rombach2021high}, we choose our baseline model to come from that class. More specifically, we follow the architecture of~\cite{blattmann2023align}, which is an extension of LDM for the video domain and has shown strong results on text-to-video modeling. Thus we take a pretrained text2image model based on StableDiffusion2.1~\footnote{\url{https://github.com/Stability-AI/stablediffusion}} and add temporal attention and convolution layer in. Compared to~\cite{blattmann2023align} our baseline differs in three aspects: First, instead of only doing temporal finetuning~\cite{blattmann2023align},  we both train the spatial and temporal layers of the latent UNet~\cite{ronneberger2015u} based denoising autoencoder. Furthermore, to limit computational demands, we train all baselines on $256 \times 256$ px resolution instead of the original $320 \times 512$ px. Finally, since we have to crop the videos most of which have non-quadratic shapes, \cf \Cref{fig:resolutions_all}, we apply size- and crop-micro-conditioning~\cite{podell2023sdxl} to be able to generate center aligned videos at inference. Exact specifications of training and sampling hyperparameters can be found in \Cref{table:hyperparameters_ablation}.

\subsection{Base Model Training and Architecture} \label{subsec:base_model_training_and_architecture}
As discussed in~\label{sec:base-model}, we start the publicly available \emph{Stable Diffusion} 2.1~\citep{rombach2021high} (SD 2.1) model. In the EDM-framework~\citep{karras2022elucidating}, SD 2.1 has the following preconditioning functions:
\begin{align}
    \cskip^\mathrm{SD 2.1}(\sigma) &= 1, \\
    \cout^\mathrm{SD 2.1}(\sigma) &= -\sigma\,, \\
    % \cin^\mathrm{SD 2.1}(\sigma) &= \left( \sigma^2 + 1 \right)^{-0.5} \\
    \cin^\mathrm{SD 2.1}(\sigma) &= \frac{1}{\sqrt{\sigma^2 + 1}}\, ,  \\
    \cnoise^\mathrm{SD 2.1}(\sigma) &= \argmin_{j \in [1000]} (\sigma - \sigma_j)\,, \\
\end{align}
where $\sigma_{j+1} > \sigma_j$. The distribution over noise levels $p(\sigma)$ used for the original SD 2.1. training is a uniform distribution over the 1000 \emph{discrete} noise levels $\{\sigma_j\}_{j \in [1000]}$. One issue with the training of SD 2.1 (and in particular its noise distribution $p(\sigma)$) is that even for the maximum discrete noise level $\sigma_{1000}$ the \emph{signal-to-noise ratio}~\citep{kingma2021variational} is still relatively high which results in issues when, for example, generating very dark images~\citep{lin2023common,guttenberg2023diffusion}. \citet{guttenberg2023diffusion} proposed \emph{offset noise}, a modification of the training objective in~\Cref{eq:diffusion_objective} by making $p(\rvn \mid \sigma)$ non-isotropic Gaussian. In this work, we instead opt to modify the preconditioning functions and distribution over training noise levels altogether. 

\textbf{Image model finetuning.} We replace the above preconditioning functions with 
\begin{align}
    \cskip(\sigma) &= \left( \sigma^2 + 1 \right)^{-1}\,, \\
    \cout(\sigma) &=  \frac{-\sigma}{\sqrt{\sigma^2 + 1}}\,, \\
    \cin(\sigma) &= \frac{1}{\sqrt{\sigma^2 + 1}}\, , \\
    \cnoise(\sigma) &= 0.25 \log \sigma, \\
\end{align}
which can be recovered in the EDM framework~\citep{karras2022elucidating} by setting $\sigma_\mathrm{data} = 1$); the preconditioning functions were originally proposed in~\citep{salimans2022progressive}. We also use the noise distribution and weighting function proposed in~\citet{karras2022elucidating}, namely $\log \sigma \sim \gN(P_\mathrm{mean}, P_\mathrm{std}^2)$ and $\lambda(\sigma) = (1 + \sigma^2) \sigma^{-2}$, with $P_\mathrm{mean}=-1.2$ and $P_\mathrm{std}=1$. We then finetune the neural network backbone $F_\vtheta$ of SD2.1 for 31k iterations using this setup. For the first 1k iterations, we freeze all parameters of $F_\vtheta$ except for the time-embedding layer and train on SD2.1's original training resolution of $512 \times 512$. This allows the model to adapt to the new preconditioning functions without unnecessarily modifying the internal representations of $F_\vtheta$ too much. Afterward, we train all layers of $F_\vtheta$ for another 30k iterations on images of size $256 \times 384$, which is the resolution used in the initial stage of video pretraining. 

\textbf{Video pretraining.} We use the resulting model as the image backbone of our video model. We then insert temporal convolution and attention layers. In particular, we follow the exact setup from~\citep{blattmann2023align}, inserting a total of 656M new parameters into the UNet bumping its total size (spatial and temporal layers) to 1521M parameters. We then train the resulting UNet on 14 frames on resolution $256\times384$ for 150k iters using AdamW~\citep{loshchilov2017decoupled} with learning rate $10^{-4}$ and a batch size of 1536. We train the model for classifier-free guidance~\citep{ho2021classifierfree} and drop out the text-conditioning 15\% of the time. Afterward, we increase the spatial resolution to $320 \times 576$ and train for an additional 100k iterations, using the same settings as for the lower-resolution training except for a reduced batch size of 768 and a shift of the noise distribution towards more noise, in particular, we increase $P_\mathrm{mean} = 0$. During training, the base model and the high-resolution Text/Image-to-Video models are all conditioned on the input video's frame rate and motion score. This allows us to vary the amount of motion in a generated video at inference time.
\subsection{High-Resolution Text-to-Video Model} \label{subsec:high_resolution_text_to_video_model}
We finetune our base model on a high-quality dataset of $\sim$ 1M samples at resolution $576 \times 1024$. We train for $50k$ iterations at a batch size of 768, learning rate $3 \times 10^{-5}$, and set $P_\mathrm{mean} = 0.5$ and $P_\mathrm{std} = 1.4$. Additionally, we track an exponential moving average of the weights at a decay rate of 0.9999. The final checkpoint is chosen using a combination of visual inspection and human evaluation.
\subsection{High-Resolution Image-to-Video Model} \label{subsec:high_resolution_image_to_video_model}
We can finetune our base text-to-video model for the image-to-video task. In particular, during training, we use one additional frame on which the model is conditioned. We do not use text-conditioning but rather replace text embeddings fed into the base model with the CLIP image embedding of the conditioning frame. Additionally, we concatenate a noise-augmented~\citep{ho2021cascaded} version of the conditioning frame channel-wise to the input of the UNet~\cite{ronneberger2015u}. In particular, we add a small amount of noise of strength $\log \sigma \sim \gN(-3.0, 0.5^2)$ to the conditioning frame and then feed it through the standard SD 2.1 encoder. The mean of the encoder distribution is then concatenated to the input of the UNet (copied across the time axis). Initially, we finetune our base model for the image-to-video task on the base resolution ($320 \times 576$) for 50k iterations using a batch size of 768 and learning rate $3 \times 10^{-5}$. Since the conditioning signal is very strong, we again shift the noise distribution towards more noise, i.e., $P_\mathrm{mean} = 0.7$ and $P_\mathrm{std} = 1.6$. Afterwards, we fintune the base image-to-video model on a high-quality dataset of $\sim$ 1M samples at $576 \times 1024$ resolution. We train two versions: one to generate 14 frames and one to generate 25 frames. We train both models for $50k$ iterations at a batch size of 768, learning rate $3 \times 10^{-5}$, and set $P_\mathrm{mean} = 1.0$ and $P_\mathrm{std} = 1.6$. Additionally, we track an exponential moving average of the weights at a decay rate of 0.9999. The final checkpoints are chosen using a combination of visual inspection and human evaluation.
\subsubsection{Linearly Increasing Guidance} We occasionally found that standard vanilla classifier-free guidance~\citep{ho2021classifierfree} (see~\Cref{eq:guidance}) can lead to artifacts: too little guidance may result in inconsistency with the conditioning frame while too much guidance can result in oversaturation. Instead of using a constant guidance scale, we found it helpful to linearly increase the guidance scale across the frame axis (from small to high). A PyTorch implementation of this novel technique can be found in~\Cref{fig:linear_pred_guidance}.
\linearpredictioncode
\subsubsection{Camera Motion LoRA}
To facilitate controlled camera motion in image-to-video generation, we train a variety of \emph{camera motion LoRAs} within the temporal attention blocks of our model~\citep{guo2023animatediff}. In particular, we train low-rank matrices of rank 16 for 5k iterations. Additional samples can be found in~\Cref{fig:additional_motion_lora}.

% \subsection{Img2Vid Details} % \label{supsec:image_to_video_details} NO SUBSECTION REF ALLOWED FOR NOW

% \subsection{Img2Vid Distillation Details} % \label{supsec:image_to_video_distilation_details} NO SUBSECTION REF ALLOWED FOR NOW

\subsection{Interpolation Model Details} 
\label{supsubsec:interpolation_model_details} 
Similar to the text-to-video and image-to-video models, we finetune our interpolation model starting from the base text-to-video model, \cf \Cref{subsec:base_model_training_and_architecture}. To enable interpolation, we reduce the number of output frames from 14 to 5, of which we use the first and last as conditioning frames, which we feed to the UNet~\citep{ronneberger2015u} backbone of our model via the concat-conditioning-mechanism~\citep{rombach2021high}. To this end, we embed these frames into the latent space of our autoencoder, resulting in two image encodings $z_s,\, z_e \in \mathbb{R}^{c \times h \times w}$, where $c=4, \,h=52, \,w=128$. To form a latent frame sequence that is of the same shape as the noise input of the UNet, \ie $\mathbb{R}^{5 \times c \times h \times w}$, we use a learned mask embedding $z_m \in\mathbb{R}^{c \times h \times w}$ and form a latent sequence $ \boldsymbol{z} = \{z_s, z_m, z_m, z_m, z_e\}\in \mathbb{R}^{5 \times c \times h \times w}$. We concatenate this sequence channel-wise with the noise input and additionally with a binary mask where 1 indicates the presence of a conditioning frame and 0 that of a mask embedding. The final input for the UNet is thus of shape $\left( 5, 9, 52, 128 \right)$. In line with previous work~\citep{ho2022imagenvideo,singer2022make,blattmann2023align}, we use noise augmentation for the two conditioning frames, which we apply in the latent space. Moreover, we replace the CLIP text representation for the crossattention conditioning with the corresponding CLIP image representation of the start frame and end frame, which we concatenate to form a conditioning sequence of length 2.  

We train the model on our high-quality dataset at spatial resolution $576 \times 1024$ using AdamW~\citep{loshchilov2017decoupled} with a learning rate of $10^{-4}$ in combination with exponential moving averaging at decay rate 0.9999 and use a shifted noise schedule with  $P_\mathrm{mean}=1$ and $P_\mathrm{std}=1.2$. Surprisingly, we find this model, which we train with a comparably small batch size of 256, to converge extremely fast and to yield consistent and smooth outputs after only 10k iterations. We take this as another evidence of the usefulness of the learned motion representation our base text-to-video model has learned.   

\subsection{Multi-view generation}

We finetuned the high-resolution image-to-video model on our specific rendering of the Objaverse dataset. We render 21 frames per orbit of an object in the dataset at $576 \times 576$ resolution and finetune the 25-frame Image-to-Video model to generate these 21 frames. We feed one view of the object as the image condition. In addition, we feed the elevation of the camera as conditioning to the model. We first pass the elevation through a timestep embedding layer that embeds the sine and cosine of the elevation angle at various frequencies and concatenates them into a vector. This vector is finally concatenated to the overall vector condition of the UNet.

We trained for 12$k$ iterations with a total batch size of 16 across 8 A100 GPUs of 80GB VRAM at a learning rate of $1 \times 10^{-5}$.
