# Supplementary material for: SV3D: Novel Multi-view Synthesis and 3D Generation from a Single Image using Latent Video Diffusion
Source: arXiv:2403.12008 source file (2024-03-18)
Supplement: Supplementary file 4 [file E.tex]

\section{Experiment Details} \label{supsec:experiment_details}

\subsection{Details on Human Preference Assessment}
\label{supsubsec:human_eval}

For most of the evaluation conducted in this paper, we employ human evaluation as we observed it to contain the most reliable signal. For text-to-video tasks and all ablations conducted for the base model, we generate video samples from a list of 64 test prompts. We then employ human annotators to collect preference data on two axes: i) visual quality and ii) prompt following. More details on how the study was conducted~\Cref{supsubsubsec:human_eval_setup} and the rankings computed~\Cref{supsubsubsec:elo_score} are listed below.

\subsubsection{Experimental Setup}
\label{supsubsubsec:human_eval_setup}

Given all models in one ablation axis (\eg four models of varying aesthetic or motion scores), we compare each prompt for each pair of models (1v1). For every such comparison, we collect on average three votes per task from different annotators, i.e., \ three each for visual quality and prompt following, respectively. Performing a complete assessment between all pair-wise comparisons gives us robust and reliable signals on model performance trends and the effect of varying thresholds.
Sample interfaces that the annotators interact with are shown in~
\Cref{fig:humanevalserver}. The order of prompts and the order between models are fully randomized. Frequent attention checks are in place to ensure data quality.

\humanevalserver

\subsubsection{Elo Score Calculation}
\label{supsubsubsec:elo_score}
To calculate rankings when comparing more than two models based on 1v1 comparisons as outlined in \Cref{supsubsubsec:human_eval_setup}, we use Elo Scores (higher-is-better)~\citep{elo1978rating}, which were originally proposed as a scoring method for chess players but have more recently also been applied to compare instruction-tuned generative LLMs~\cite{bai2022training,askell2021general}. For a set of competing players with initial ratings $R_{\text{init}}$ participating in a series of zero-sum games, the Elo rating system updates the ratings of the two players involved in a particular game based on the expected and actual outcome of that game. Before the game with two players with ratings $R_1$ and $R_2$, the expected outcome for the two players is calculated as
\begin{align}
\label{eq:expected_elo}
E_1 =  \frac{1}{1 + 10^{\frac{R_2 - R_1}{400}}} \, , \\
E_2 =  \frac{1}{1 + 10^{\frac{R_1 - R_2}{400}}} \, . 
\end{align}
After observing the result of the game, the ratings $R_i$ are updated via the rule
\begin{align}
\label{eq:ranking_update}
R^{'}_{i} =  R_i + K \cdot \left(S_i - E_i \right), \quad i \in \{1,2\}
\end{align}
where $S_i$ indicates the outcome of the match for player $i$. In our case, we have $S_i=1$ if player $i$ wins and $S_i = 0$ if player $i$ loses. The constant $K$ can be seen as weight emphasizing more recent games. We choose $K=1$ and bootstrap the final Elo ranking for a given series of comparisons based on 1000 individual Elo ranking calculations in a randomly shuffled order. Before comparing the models, we choose the start rating for every model as $R_{\text{init}} = 1000$.

\subsection{Details on Experiments from \Cref{sec:approach}} 
 
\subsubsection{Architectural Details}
Architecturally, all models trained for the presented analysis in \Cref{sec:approach} are identical. To insert create a temporal UNet~\citep{ronneberger2015u} based on an existing spatial model, we follow \citet{blattmann2023align} and add temporal convolution and (cross-)attention layers after each corresponding spatial layer. As a base 2D-UNet, we use the architecture from \emph{Stable Diffusion 2.1}, whose weights we further use to initialize the spatial layers for all runs except the second one presented in \Cref{fig:imageonly_comp}, where we intentionally skip this initialization to create a baseline for demonstrating the effect of image-pretraining. 
Unlike \citet{blattmann2023align}, we train all layers, including the spatial ones, and do not freeze the spatial layers after initialization. All models are trained with the AdamW~\citep{loshchilov2017decoupled} optimizer with a learning rate of $1.e-4$ and a batch size of $256$. Moreover, in contrast to our models from \Cref{sec:sota}, we do not translate the noise process to continuous time but use the standard linear schedule used in \emph{Stable Diffusion 2.1}, including offset noise~\citep{guttenberg2023diffusion}, in combination with the v-parameterization~\citep{ho2022classifier}. We omit the text-conditioning in 10\% of the cases to enable classifier-free guidance~\citep{ho2022classifier} during inference. 
To generate samples for the evaluations, we use 50 steps of the deterministic DDIM sampler~\citep{song2020improved} with a classifier guidance scale of 12 for all models. 

\subsubsection{Calibrating Filtering Thresholds}
\label{supsubsec:filtering_ablations}
\smallscaleablations
Here, we present the outcomes of our study on filtering thresholds presented in \Cref{subsec:data_curation}. As stated there, we conduct experiments for the optimal filtering threshold for each type of annotation while not filtering for any other types. The only difference here is our assessment of the most suitable captioning method, where we simply compare all used captioning methods. We train each model on videos consisting of 8 frames at resolution $256 \times 256$ for exactly 40k steps with a batch size of 256, roughly corresponding to 10M training examples seen during training. For evaluation, we create samples based on 64 pre-selected prompts for each model and conduct a human preference study as detailed in \Cref{supsubsec:human_eval}. \Cref{fig:filtering_ablations} shows the ranking results of these human preference studies for each annotation axis for spatiotemporal sample quality and prompt following. Additionally, we show an averaged `aggregated' score. 

For \emph{captioning}, we see that - surprisingly - the captions generated by the simple clip-based image captioning method CoCa of \citet{yu2022coca} clearly have the most beneficial influence on the model. However, since recent research recommends using more than one caption per training example, we sample one of the three distinct captions during training. We nonetheless reflect the outcome of this experiment by shifting the captioning sampling distribution towards CoCa captions by using $p_{\text{CoCa}} = 0.5; \, p_{\text{V-BLIP}} = 0.25; \,p_{\text{LLM}} = 0.25; \,$.

For \emph{motion filtering}, we choose to filter out 25\% of the most static examples. However, the aggregated preference score of the model trained with this filtering method does not rank as high in human preference as the non-filtered score. The rationale behind this is that non-filtered ranks best primarily because it ranks best in the category `prompt following' which is less important than the `quality' category when assessing the effect of motion filtering. Thus, we choose the 25\% threshold, as mentioned above, since it achieves both competitive performances in `prompt following' and `quality'. 

For \emph{aesthetics filtering}, where, as for motion thresholding, the `quality' category is more important than the `prompt following'-category, we choose to filter out the 25 \% with the lowest aesthetics score, while for \emph{CLIP-score thresholding} we omit even 50\% since the model trained with the corresponding threshold is performing best. Finally, we filter out the 25\% of samples with the largest text area covering the videos since it ranks highest both in the `quality' category and on average.

Using these filtering methods, we reduce the size of \dataset by more than a factor of 3, \cf \Cref{tab:subset_stats}, but obtain a much cleaner dataset as shown in \Cref{sec:approach}. For the remaining experiments in \Cref{subsec:data_curation}, we use the identical architecture and hyperparameters as stated above. We only vary the dataset as detailed in \Cref{subsec:data_curation}.

\subsubsection{Finetuning Experiments}
\label{supsubsec:finetune_exps}
For the finetuning experiments shown in \Cref{subsec:stage3}, we again follow the architecture, training hyperparameters, and sampling procedure stated at the beginning of this section. The only notable differences are the exchange of the dataset and the increase in resolution from the pretraining resolution $256 \times 256$ to $512 \times 512$ while still generating videos consisting of 8 frames. We train all models presented in this section for 50k steps.

\subsection{Human Eval vs SOTA}

For comparison of our image-to-video model with state-of-the-art models like Gen-2~\cite{gen2} and Pika~\cite{pika}, we randomly choose 64 conditioning images generated from a $1024 \times 576$ finetune of SDXL~\cite{podell2023sdxl}. We employ the same framework as in~\Cref{supsubsubsec:human_eval_setup} to evaluate and compare the visual quality generated samples with other models. 

For Gen-2, we sample the image-to-video model from the web UI. We fixed the same seed of 23, used the default motion value of 5 (on a scale of 10), and turned on the ``Interpolate" and ``Remove watermark" features. This results in 4-second samples at $1408 \times 768$. We then resize the shorter side to yield $1056 \times 576$ and perform a center-crop to match our resolution of $1024 \times 576$. For our model, we sample our 25-frame image-to-video finetune to give 28 frames and also interpolate using our interpolation model to yield samples of 3.89 seconds at 28 FPS. We crop the Gen-2 samples to 3.89 seconds to avoid biasing the annotators.

For Pika, we sample the image-to-video model from the Discord bot. We fixed the same seed of 23, used the motion value of 2 (on a scale of 0-4), and specified a 16:9 aspect ratio. This results in 3-second samples at $1024 \times 576$, which matches our resolution. For our model, we sample our 25-frame image-to-video finetune to give 28 frames and also interpolate using our interpolation model to yield samples of 3.89 seconds at 28 FPS. We crop our samples to 3 seconds to match Pika and avoid biasing the annotators. Since Pika samples have a small ``Pika Labs" watermark in the bottom right, we pad that region with black pixels for both Pika and our samples to also avoid bias.

% \todo{Needs details on exact questions etc, maybe take a look at VideoLDM paper, we even showed screenshots there} 

\subsection{UCF101 FVD} \label{supsec:ucf101_fvd}
This section describes the zero-shot UCF101 FVD computation of our base text-to-video model. The UCF101 dataset~\citep{soomro2012ucf101} consists of 13,320 video clips, which are classified into 101 action categories. All videos are of frame rate 25 FPS and resolution $240\times320$. To compute FVD, we generate 13,320 videos (16 frames at 25 FPS, classifier-free guidance with scale $w=7$) using the same distribution of action categories, that is, for example, 140 videos of ``TableTennisShot'', 105 videos of ``PlayingPiano'', etc. We condition the model directly on the action category (``TableTennisShot'', ``PlayingPiano'', etc.) and do not use any text modification. Our samples are generated at our model's native resolution $320 \times 576$ (16 frames), and we downsample to $240 \times 432$ using bilinear interpolation with antialiasing, followed by a center crop to $240 \times 320$. We extract features using a pretrained I3D action classification model~\citep{carreira2017quo}, in particular we are using a torchscript\footnote{\url{https://www.dropbox.com/s/ge9e5ujwgetktms/i3d_torchscript.pt} with keyword arguments \texttt{rescale=True, resize=True, return\_features=True}.} provided by~\citet{brooks2022generating}.

\subsection{Additional Samples}
Here, we show additional samples for the models introduced in \Cref{sec:base-model,sec:txt2vid,sec:img2vid,sec:multiview}.

\subsubsection{Additional Text-to-Video Samples}
\additionaltexttwovideo
In \Cref{fig:additional_txt2vid}, we show additional samples from our text-to-video model introduced in~\Cref{sec:txt2vid}.
\subsubsection{Additional Image-to-Video Samples}
\additionalimagetwovideo
In \Cref{fig:additional_img2vid}, we show additional samples from our image-to-video model introduced in \Cref{sec:img2vid}.
\subsubsection{Additional Camera Motion LoRA Samples}
\additionalmotionlora
In \Cref{fig:additional_motion_lora}, we show additional samples for our motion LoRA's tuned for camera control as presented in \Cref{subsec:motion_lora}.
\subsubsection{Temporal Prompting via Temporal Cross-Attention Layers}
\additionaltemporalattention
Our architecture follows \citet{blattmann2023align}, who introduced dedicated temporal cross-attention layers, which are used interleaved with the spatial cross-attention layers of the standard 2D-UNet~\citep{dhariwal2021diffusion,ho2020ddpm}. During probing our Text-to-Video model from \Cref{sec:txt2vid}, we noticed that it is possible to independently prompt the model spatially and temporally by using different text-prompts as inputs for the spatial and temporal cross-attention conditionings, see \Cref{fig:additional_temporal_attention}. To achieve this, we use a dedicated spatial prompt to describe the general content of the scene to be depicted while the motion of that scene is fed to the model via a separate temporal prompt, which is the input to the temporal cross-attention layers. We provide an example of these first experiments indicating this implicit disentanglement of motion and content in \Cref{fig:additional_temporal_attention}, where we show that varying the temporal prompt while fixing random seed and spatial prompt leads to spatially similar scenes that obtain global motion properties following the temporal prompt.       

\subsubsection{Additional Samples on Multi-View Synthesis}
In \Cref{fig:additional_mv1,fig:additional_mv2,fig:additional_mv3,fig:additional_mv4}, we show additional visual examples for SVD-MV, trained on our renderings of Objaverse and MVImageNet datasets as described in \Cref{sec:multiview}.
\MVIone
\MVItwo
\MVIthree
\MVIfour

% \label{subsec:poseobjaverse}

% TIM Killed this section for now, make subsection in experiment details instead
% \section{Multi-view generation}
% \label{sec:MV}
